# Supplementary material for: Some open mathematical problems on fullerenes
Source: arXiv:2410.19322 source file (2024-10-25)
Supplement: Supplementary file 1 [file 07_appendix.tex]

\section*{Appendix}\label{section:appendix}

\begin{construction}\label{construction:50--nanotube}
A finite dual $(5,0)$--nanotube can be constructed by combining two copies of the cap shown on the left of Figure \ref{fig:N50_construction}, with $r\in\N_0$ hexagonal belts, as depicted on the right in Figure \ref{fig:N50_construction}. 
Each cap contains six vertices of degree $5$ and no vertex of degree $6$. 
The hexagonal ring consists of $5$ vertices.
Therefore, for a finite dual  $(5,0)$--nanotube with $r$ hexagonal rings, the total number of vertices in the original fullerene is given by $n = 20 + 10r$.

\begin{figure}[H]
\begin{center}
\includegraphics[scale=1.2]{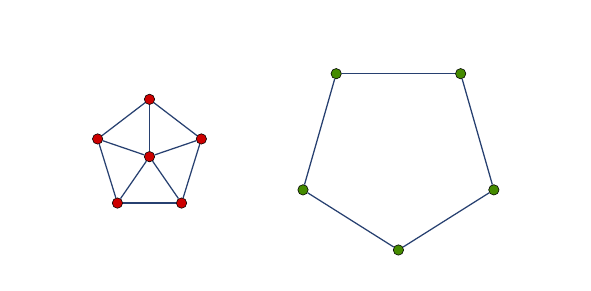}
\caption{Left: Cap of a finite dual $(5,0)$--nanotube. Right: (Dual) Hexagonal ring, which can be appended arbitrarily often to the cap.}\label{fig:N50_construction}
\end{center}
\end{figure}
For $r=0$, i.e. without any hexagonal ring and representing the smallest possible finite $(5,0)$--nanotube, the two caps can be directly connected, as shown in Figure \ref{figure:C20_c30_cconstruction}, resulting in the dodecahedron $C_{20}$.
\begin{figure}[H]
\begin{center}
\includegraphics[scale=0.75]{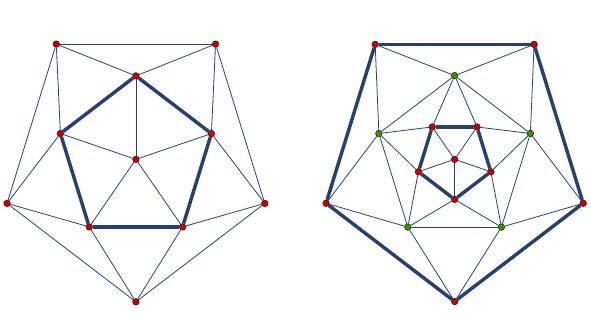}
\caption{Dual graphs of facets of the dodecahedron and $C_{30,1}$ ($(5,0)$-nanotube with $r=1$ hexagonal ring), highlighting two copies of the cap shown in Figure \ref{fig:N50_construction}. 
The outer edges of the two caps are shown with thicker lines.}\label{figure:C20_c30_cconstruction}
\end{center}
\end{figure}
\end{construction}

%\begin{construction}\label{construction:55--nanotube}
%A finite dual $(5,5)$--nanotube can be constructed by combining two copies of the cap shown on the left of Figure \ref{fig:N55_construction}, with $r\in\N_0$ hexagonal belts, as depicted on the right in Figure \ref{fig:N55_construction}. 
%Each cap contains six vertices of degree $5$ and ten vertices of degree $6$. 
%The hexagonal ring consists of $10$ vertices.
%Therefore, for a finite dual  $(5,5)$--nanotube with $r$ hexagonal rings, the total number of vertices in the original fullerene is given by
%\begin{align*}
%n = 60 + 20r.
%\end{align*}

%\begin{figure}[H]
%\begin{center}
%\includegraphics[scale=1.2]{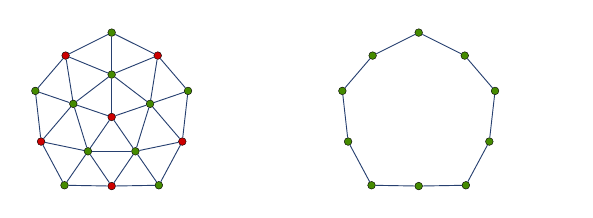}
%\caption{Left: Cap of a finite dual $(5,5)$--nanotube. Right: (Dual) Hexagonal ring, which can be appended arbitrarily often to the cap.}\label{fig:N55_construction}
%\end{center}
%\end{figure}
%For $r=0$, i.e. without any hexagonal ring and representing the smallest possible finite $(5,5)$--nanotube, the two caps can be directly connected, as shown in Figure \ref{figure:C60_caps}, resulting in the \textit{Buckminster fullerene} $C_{60,1812}$.
%\begin{figure}[H]
%\begin{center}
%\includegraphics[scale=0.35]{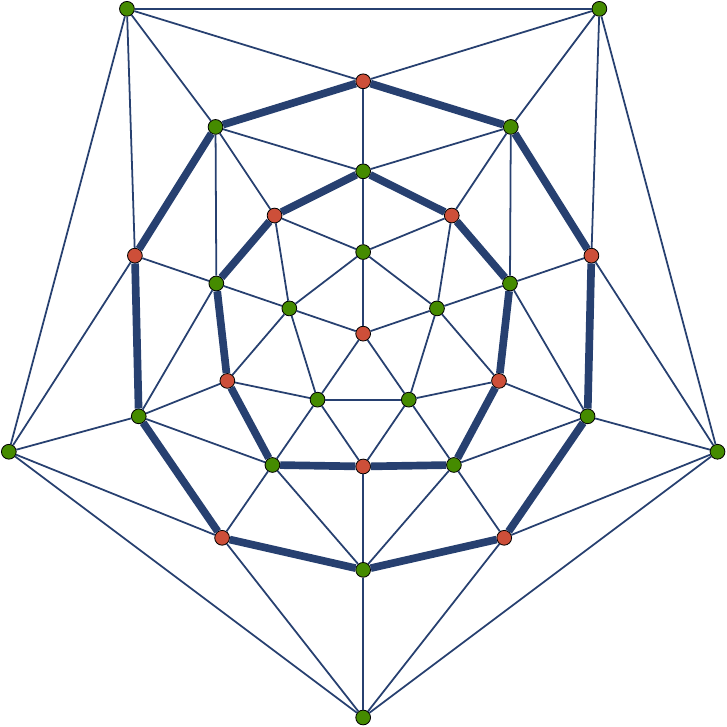}
%\caption{Dual graph of the Buckminster fullerene, highlighting two copies of the cap shown in Figure \ref{fig:N55_construction}. The outer edges of the two caps are shown with thicker lines.}\label{figure:C60_caps}
%\end{center}
%\end{figure}
%\end{construction}
